# Supplementary material for: Circuit QED with Hole-Spin Qubits in Ge/Si Nanowire Quantum Dots
Source: arXiv:1306.3596 source file (2013-12-12)
Supplement: Supplementary file 1 [file Kloeffel_Supplement_Nov2013.pdf]

# Supplementary information to “Circuit QED with hole-spin qubits in Ge/Si nanowire quantum dots”

Christoph Kloeffel,<sup>1</sup> Mircea Trif,<sup>2</sup> Peter Stano,<sup>1,3,4</sup> and Daniel Loss<sup>1,4</sup>

<sup>1</sup>*Department of Physics, University of Basel, Klingelbergstrasse 82, CH-4056 Basel, Switzerland*

<sup>2</sup>*Department of Physics and Astronomy, University of California, Los Angeles, California 90095, USA*

<sup>3</sup>*Institute of Physics, Slovak Academy of Sciences, 845 11 Bratislava, Slovakia*

<sup>4</sup>*CEMS, RIKEN, Wako, Saitama 351-0198, Japan*

(Dated: November 18, 2013)

## I. EFFECTIVE 1D HAMILTONIAN

### Basis states

The low-energy hole states in a Ge/Si core/shell nanowire (NW) are well described by the effective 1D Hamiltonian derived in Ref. [1]. Using the notation introduced therein, with the NW axis referred to as the  $z$  axis, the four basis states that comprise the spin and the transverse subband degrees of freedom read

$$|g_+\rangle = \left( a_g J_2(k_{\text{hh}}^g r) + \sqrt{3} b_g J_2(k_{\text{lh}}^g r) \right) e^{-2i\phi} |3/2\rangle + \left( b_g J_0(k_{\text{lh}}^g r) - \sqrt{3} a_g J_0(k_{\text{hh}}^g r) \right) |-1/2\rangle, \quad (1)$$

$$|g_-\rangle = \left( a_g J_2(k_{\text{hh}}^g r) + \sqrt{3} b_g J_2(k_{\text{lh}}^g r) \right) e^{2i\phi} |-3/2\rangle + \left( b_g J_0(k_{\text{lh}}^g r) - \sqrt{3} a_g J_0(k_{\text{hh}}^g r) \right) |1/2\rangle, \quad (2)$$

$$|e_+\rangle = -a_e J_1(k_{\text{hh}}^e r) \left( e^{-i\phi} |3/2\rangle + \sqrt{3} e^{i\phi} |-1/2\rangle \right), \quad (3)$$

$$|e_-\rangle = a_e J_1(k_{\text{hh}}^e r) \left( e^{i\phi} |-3/2\rangle + \sqrt{3} e^{-i\phi} |1/2\rangle \right), \quad (4)$$

where the  $J_i(\kappa)$  with integer  $i$  are Bessel functions of the first kind. The polar coordinates  $r$  and  $\phi$  in the cross section are related to the cartesian coordinates by  $x = r \cos \phi$  and  $y = r \sin \phi$  (origin on the symmetry axis of the NW). The  $|m_z\rangle$ ,  $m_z \in \{\pm 3/2, \pm 1/2\}$ , correspond to the effective electron spin states in the topmost valence band (VB) and fulfill  $J_z |m_z\rangle = m_z |m_z\rangle$ , where  $J_z$  is the operator for the  $z$ -projection of this effective spin 3/2. The wave numbers  $k_{\text{hh}}^g, k_{\text{lh}}^g, k_{\text{hh}}^e$  and the coefficients  $a_g, b_g, a_e$  are determined by the Luttinger parameters of Ge and result from the hard-wall boundary conditions at the Ge/Si interface and the normalization. We choose all coefficients as real, with  $a_g < 0, b_g > 0$ , and  $a_e > 0$ . For further details, see Ref. [1].

### Effective 1D Hamiltonian

In the setup studied in the main text, we consider a magnetic field  $B_y$  along the  $y$  axis and electric fields  $E_y$  and  $E_z$  along the  $y$  and  $z$  axes, respectively. For the externally controlled electric-dipole-induced spin resonance (EDSR), we assume  $E_z = E_z(t) = E_{z,0}^c \cos(\omega_{\text{act}} t)$  with amplitude  $E_{z,0}^c$  and angular frequency  $\omega_{\text{act}}$ . The quantized field of the cavity is described by  $E_z = E_{z,0}^c (a^\dagger + a)$ , see also Sec. V, where  $E_{z,0}^c$

is the amplitude and  $a^\dagger$  ( $a$ ) is the bosonic creation (annihilation) operator for the cavity mode that is near or at resonance with the qubit. The different contributions to the Hamiltonian

$$H = H_{\text{LK}} + H_{\text{BP}} + H_B + H_{\text{DR}} + H_{\text{R},y} + H_{\text{R},z} - eE_z z + V(z) \quad (5)$$

for this setup take the following  $4 \times 4$  representation when written out explicitly in the basis  $\Sigma_{1\text{D}} = \{g_+, g_-, e_+, e_-\}$ . First,

$$H_{\text{LK}} + H_{\text{BP}} = \begin{pmatrix} \frac{\hbar^2 k_z^2}{2m_g} & 0 & 0 & -iCk_z \\ 0 & \frac{\hbar^2 k_z^2}{2m_g} & -iCk_z & 0 \\ 0 & iCk_z & \frac{\hbar^2 k_z^2}{2m_e} + \Delta & 0 \\ iCk_z & 0 & 0 & \frac{\hbar^2 k_z^2}{2m_e} + \Delta \end{pmatrix} \quad (6)$$

combines the Luttinger-Kohn (LK) and the Bir-Pikus (BP) Hamiltonian, where the latter changes the energy gap  $\Delta = \Delta_{\text{LK}} + \Delta_{\text{BP}}(\gamma)$  through the static strain that is caused by the Si shell of relative thickness  $\gamma$ . The latter is defined as  $\gamma = (R_s - R)/R$ , where  $R$  ( $R_s$ ) is the core (shell) radius. Second,

$$H_B = \mu_B B_y \begin{pmatrix} 0 & iK & Lk_z & 0 \\ -iK & 0 & 0 & -Lk_z \\ Lk_z & 0 & 0 & -iM \\ 0 & -Lk_z & iM & 0 \end{pmatrix} \quad (7)$$

describes the orbital and Zeeman-type coupling due to  $B_y$ . Third,

$$H_{\text{DR}} = eE_y U \begin{pmatrix} 0 & 0 & i & 0 \\ 0 & 0 & 0 & i \\ -i & 0 & 0 & 0 \\ 0 & -i & 0 & 0 \end{pmatrix} \quad (8)$$

is the direct Rashba spin-orbit interaction (DRSOI) induced by  $E_y$ , and the conventional Rashba spin-orbit interaction (RSOI) reads

$$H_{\text{R},y} = \alpha E_y \begin{pmatrix} 0 & Tk_z & iS & 0 \\ Tk_z & 0 & 0 & iS \\ -iS & 0 & 0 & -\frac{3}{4}k_z \\ 0 & -iS & -\frac{3}{4}k_z & 0 \end{pmatrix}. \quad (9)$$

Finally, one finds

$$H_{\text{R},z} = 2\alpha E_z S \begin{pmatrix} 0 & 0 & 0 & 1 \\ 0 & 0 & 1 & 0 \\ 0 & 1 & 0 & 0 \\ 1 & 0 & 0 & 0 \end{pmatrix} \quad (10)$$

for the RSOI due to  $E_z$ . In the main text, we write  $H_R = H_{R,y} + H_{R,z}$  for brevity. The longitudinal confinement  $V(z)$  and the linear shift  $-eE_z z$  do not affect the states  $|g_{\pm}\rangle$ ,  $|e_{\pm}\rangle$ , and therefore come with the identity matrix in this basis. We note that  $H_{DR}$  is obtained by projecting the direct coupling to the hole charge,  $-eE_y y$ , onto the low-energy subspace, whereas  $H_{R,y}$  and  $H_{R,z}$  result from  $\alpha E_y (k_z J_x - k_x J_z)$  and  $\alpha E_z (k_x J_y - k_y J_x)$ , respectively. Here,  $e$  is the elementary positive charge,  $\alpha$  is a material-dependent constant  $\propto (\text{band gap})^{-2}$  [2], and  $\hbar k_i$  ( $\hbar J_i$ ) is the operator for the momentum (spin) along the  $i$  axis. Further information on the different contributions can be found in Ref. [1], and the values of all relevant constants are summarized in Table I.

TABLE I. Constants in the 1D model for holes in Ge/Si nanowires. The values were calculated as explained in Ref. [1] and in the text;  $\alpha$  was obtained following Ref. [2], and underlying Luttinger parameters for Ge were taken from Ref. [3].  $R$  denotes the core radius,  $m$  is the bare electron mass, and  $e$  is the elementary positive charge.

| Constant | Value                 | Constant      | Value                   |
|----------|-----------------------|---------------|-------------------------|
| $C$      | $7.26 \hbar^2 / (mR)$ | $\Delta_{LK}$ | $0.73 \hbar^2 / (mR^2)$ |
| $m_g$    | $0.043 m$             | $m_e$         | $0.054 m$               |
| $K$      | $2.89$                | $L$           | $8.04 R$                |
| $M$      | $2.56$                | $U$           | $0.15 R$                |
| $S$      | $0.36/R$              | $T$           | $0.98$                  |
| $\alpha$ | $-0.4 \text{ nm}^2 e$ |               |                         |

## II. QUANTUM DOT: PERTURBATIVE ANALYSIS

### Hamiltonian

In the presence of harmonic confinement

$$V(z) = \frac{m_g \omega_g^2 z^2}{2} = \frac{\hbar \omega_g z^2}{2 l_g^2}, \quad (11)$$

where the confinement length

$$l_g = \sqrt{\frac{\hbar}{m_g \omega_g}} \quad (12)$$

is defined by the effective mass  $m_g$  and the associated level spacing  $\hbar \omega_g$ , we now derive an effective  $2 \times 2$  Hamiltonian

$$H_q = \frac{E_Z}{2} \tilde{\sigma}_z + T_q \tilde{\sigma}_x \quad (13)$$

for qubits that are formed by the two hole states of lowest energy in the quantum dot (QD). Here, the  $\tilde{\sigma}_i$  are spin-1/2 Pauli operators, and the tilde denotes that they act on the two QD states that form the qubit, in contrast to the  $\sigma_i$  that act on the spin index  $\{+, -\}$ . The parameters in  $H_q$  are the Zeeman splitting  $E_Z$  and the transverse coupling  $T_q \propto E_z$  that is induced by the electric field along the NW. Writing  $T_q = \bar{\nu} E_z$ , one has  $T_q = \nu_e \cos(\omega_{act})$  for externally driven EDSR, and  $T_q = \nu_c (a^\dagger + a)$  for the cavity field. The coupling strengths

$\nu_{e,c} = \bar{\nu} E_{z,0}^{e,c}$  are proportional to the amplitudes  $E_{z,0}^{e,c}$ , and we calculate the proportionality factor  $\bar{\nu}$  below. Without loss of generality,  $E_Z$  and  $\bar{\nu}$  will always be defined as positive. Because typical Ge/Si NWs are rather thin,  $R \sim 5\text{--}10$  nm, we consider elongated QDs with  $l_g \gg R$ . This implies that the hole states are very well described by  $H$ , Eq. (5), where the effective 1D Hamiltonian is supplemented with the confinement  $V(z)$ . We now derive an analytical expression for  $H_q$  perturbatively.

From numerical results, Sec. III, we find that  $H_{R,z}$  and the difference between  $m_g$  and  $m_e$  may be neglected to a very good accuracy. Within the perturbative analysis, we therefore omit  $H_{R,z}$  and set  $m_g = m_e \equiv m_g$  for simplicity. The part of  $H$ , Eq. (5), that comes with the identity matrix in the basis  $\Sigma_{1D}$  then reads

$$H^{\text{id}} = \frac{\hbar^2 k_z^2}{2m_g} - eE_z z + V(z). \quad (14)$$

With the definition

$$U' \equiv U + \alpha S / e, \quad (15)$$

the remaining terms of  $H$  may be written as  $H_{1D}^a + H_{1D}^b + H_B$ , where

$$H_{1D}^a = \begin{pmatrix} 0 & 0 & ieE_y U' & 0 \\ 0 & 0 & 0 & ieE_y U' \\ -ieE_y U' & 0 & \Delta & 0 \\ 0 & -ieE_y U' & 0 & \Delta \end{pmatrix} \quad (16)$$

and

$$H_{1D}^b = k_z \begin{pmatrix} 0 & \alpha E_y T & 0 & -iC \\ \alpha E_y T & 0 & -iC & 0 \\ 0 & iC & 0 & -\frac{3}{4}\alpha E_y \\ iC & 0 & -\frac{3}{4}\alpha E_y & 0 \end{pmatrix}. \quad (17)$$

### Step 1

For Ge/Si NWs with typically  $R \sim 5\text{--}10$  nm and  $\gamma \sim 10\%\text{--}50\%$ , one finds  $10 \text{ meV} \lesssim \Delta \lesssim 25 \text{ meV}$ . Although this energy scale is rather large, we want to derive an effective model that also applies for rather strong electric fields for which  $|eE_y U'| \sim \Delta$ . Therefore, we first perform a unitary transformation

$$H' = U_1^\dagger H U_1 = H^{\text{id}} + H_{1D}^{\prime a} + U_1^\dagger (H_{1D}^b + H_B) U_1, \quad (18)$$

where the transformation matrix

$$U_1 = \begin{pmatrix} \cos \theta & 0 & i \sin \theta & 0 \\ 0 & \cos \theta & 0 & i \sin \theta \\ i \sin \theta & 0 & \cos \theta & 0 \\ 0 & i \sin \theta & 0 & \cos \theta \end{pmatrix} \quad (19)$$

brings  $H_{1D}^a$  into the diagonal form

$$H_{1D}^{\prime a} = U_1^\dagger H_{1D}^a U_1 = \begin{pmatrix} 0 & 0 & 0 & 0 \\ 0 & 0 & 0 & 0 \\ 0 & 0 & \Delta' & 0 \\ 0 & 0 & 0 & \Delta' \end{pmatrix}. \quad (20)$$

Above, we neglect global shifts in energy and use

$$\cos \theta \equiv \frac{\Delta + \Delta'}{\sqrt{(\Delta + \Delta')^2 + (2eE_y U')^2}}, \quad (21)$$

$$\sin \theta \equiv \frac{2eE_y U'}{\sqrt{(\Delta + \Delta')^2 + (2eE_y U')^2}}, \quad (22)$$

$$\Delta' \equiv \sqrt{\Delta^2 + (2eE_y U')^2}. \quad (23)$$

We note that  $U_1$  and  $H_{1D}^a$  in Eqs. (19) and (20) are represented in the basis  $\Sigma_{1D}$  introduced before. That is, we keep the basis states fixed and rearrange the matrix elements according to  $U_1$ . Although  $H' \neq H$  in general,  $H$  can, of course, be represented in exactly the same quasi-diagonal form as  $H'$ , as the inverse transformation  $H = U_1 H' U_1^\dagger$  may be performed by changing the basis states while keeping the matrix elements the same. In the proposed setup, knowledge of the eigenstates that form the qubit is not required (see end of this section). Therefore, we proceed analogously with the remaining unitary transformations, i.e., we keep the basis states fixed and work with the formally equivalent, rotated versions of the Hamiltonian. If needed, the basis states of the unrotated system may be calculated either numerically (see Sec. III) or via inverse transformations as mentioned above.

### Step 2

The second unitary transformation corresponds to a Schrieffer-Wolff (SW) transformation that perturbatively decouples  $|g_\pm\rangle$  from  $|e_\pm\rangle$  to second order, where  $\Delta'$  in  $H_{1D}^a$  provides the large energy. When the SW transformation is formally denoted by  $U_2$ , we find

$$H_g = P_g U_2^\dagger H' U_2 P_g = H_g^0 + H_g^r \quad (24)$$

for the projection ( $P_g$ ) onto the subspace  $\Sigma_g = \{g_+, g_-\}$  of the bands of lowest-energy, where

$$H_g^0 = \begin{pmatrix} \frac{\hbar^2 k_z^2}{2m_g'} + V(z) & C' k_z + iE_{Z,g}^0/2 \\ C' k_z - iE_{Z,g}^0/2 & \frac{\hbar^2 k_z^2}{2m_g'} + V(z) \end{pmatrix} \quad (25)$$

contains the dominant contributions and  $H_g^r$  contains the rest. In Eq. (25), the shorthand notation

$$E_{Z,g}^0 \equiv 2\mu_B B_y (K \cos^2 \theta - M \sin^2 \theta) \quad (26)$$

stands for the Zeeman splitting at  $k_z = 0$ , and

$$m_g' = \left( \frac{1}{m_g} - \frac{2\tilde{C}^2}{\hbar^2 \Delta'} \right)^{-1} \quad (27)$$

is the corrected effective mass, where

$$\tilde{C} \equiv C \cos(2\theta) - \alpha E_y \frac{3 + 4T}{8} \sin(2\theta). \quad (28)$$

Due to the large coupling constants  $C$  and  $U$ , the expression

$$C' \equiv C \sin(2\theta) + \alpha E_y \left( T \cos^2 \theta - \frac{3}{4} \sin^2 \theta \right) \quad (29)$$

in Eq. (25) becomes large even at moderate  $E_y$ , so that  $C' k_z$  is no longer a small perturbation when the applied field exceeds a certain threshold value. In typical Ge/Si NW QDs, one finds  $|C'|/l_g \sim \hbar\omega_g$  for  $|E_y| \sim 1 \text{ V}/\mu\text{m}$ , and we therefore treat this coupling as part of the leading-order Hamiltonian.

### Step 3

Next, we introduce a suitable basis for the QD states. For this, we consider the Hamiltonian

$$H_g' = U_3^\dagger H_g U_3 = H_g'^0 + H_g'^r, \quad (30)$$

where

$$U_3 = \frac{1}{\sqrt{2}} \begin{pmatrix} 1 & -1 \\ 1 & 1 \end{pmatrix} \quad (31)$$

was chosen such that  $H_g'^0 = U_3^\dagger H_g^0 U_3$  reads

$$H_g'^0 = \frac{\hbar^2 k_z^2}{2m_g'} + V(z) + \begin{pmatrix} C' k_z & iE_{Z,g}^0/2 \\ -iE_{Z,g}^0/2 & -C' k_z \end{pmatrix}. \quad (32)$$

We note that

$$\frac{\hbar^2 k_z^2}{2m_g'} \pm C' k_z = \frac{\hbar^2}{2m_g'} \left( k_z \pm \frac{C' m_g'}{\hbar^2} \right)^2 - \frac{C'^2 m_g'}{2\hbar^2}, \quad (33)$$

and from the diagonal elements of Eq. (32) we identify

$$|n_\pm\rangle \equiv |g_\pm\rangle \otimes e^{\mp i C' m_g' z / \hbar^2} |\varphi_n\rangle \quad (34)$$

as a well-suited set of basis states for  $H_g'$ . The  $|\varphi_n\rangle$ , with quantum number  $n \in \{0, 1, \dots\}$ , correspond to the solutions  $\varphi_n(z)$  of the 1D harmonic oscillator

$$\left( \frac{\hbar^2 k_z^2}{2m_g'} + V(z) \right) \varphi_n(z) = \hbar\omega_g' \left( n + \frac{1}{2} \right) \varphi_n(z), \quad (35)$$

where  $k_z = -i\partial_z$  in coordinate space. The effective level spacing reads

$$\hbar\omega_g' = \sqrt{\frac{m_g}{m_g'}} \hbar\omega_g \quad (36)$$

and, consequently, one may define the corrected confinement length  $l_g'$  as

$$l_g' = \sqrt{\frac{\hbar}{m_g' \omega_g'}} = l_g \left( \frac{m_g}{m_g'} \right)^{1/4}. \quad (37)$$

We mention in passing that  $H_g^r$  and  $H_g'^r$  contain a term  $\propto B_y^2 k_z^2$  that gives rise to additional rescaling of the effective

mass. Taking this term into account, the corrected effective mass reads

$$m_g'' = \left( \frac{1}{m_g} - \frac{2\tilde{C}^2 + 2(\mu_B L B_y)^2}{\hbar^2 \Delta'} \right)^{-1}, \quad (38)$$

which implies that the level spacing depends on both  $E_y$  and  $B_y$ . However, the above correction due to  $B_y$  turns out to be very small, and we therefore treat this term as part of  $H_g''$ .

Using

$$\left( \frac{\hbar^2 k_z^2}{2m_g'} + V(z) \pm C' k_z \right) |n_{\pm}\rangle = E_n |n_{\pm}\rangle, \quad (39)$$

with

$$E_n = \hbar\omega_g' \left( n + \frac{1}{2} \right) - \frac{C'^2 m_g'}{2\hbar^2}, \quad (40)$$

we represent  $H_g'$  by a  $2N$ -dimensional matrix with basis

$$\Sigma_N = \{0_+, 0_-, \dots, (N-1)_+, (N-1)_-\}. \quad (41)$$

The projection onto this basis is denoted by  $P_N^{\text{QD}}$ , and the projected versions of  $H_g'$ ,  $H_g^0$ , and  $H_g''$  are referred to as

$$H_N = P_N^{\text{QD}} H_g' P_N^{\text{QD}}, \quad (42)$$

$$H_N^0 = P_N^{\text{QD}} H_g^0 P_N^{\text{QD}}, \quad (43)$$

$$H_N'' = P_N^{\text{QD}} H_g'' P_N^{\text{QD}}. \quad (44)$$

We note that  $H_N = H_g'$  in the limit  $N \rightarrow \infty$  (analogously for  $H_N^0$  and  $H_N''$ ). As discussed below, we find that  $N = 3$  is usually sufficient for a quantitatively reliable estimate of  $H_q$ , Eq. (13).

#### Step 4

A fourth unitary transformation is required to derive a leading-order Hamiltonian  $H_N^a$  that is diagonal and includes the Zeeman splitting. This Hamiltonian is calculated via

$$H_N^a = \text{Diagonal}[U_4^\dagger H_N^0 U_4], \quad (45)$$

where  $\text{Diagonal}[A]$  stands for the diagonal part of matrix  $A$ . The transformation matrix  $U_4$  corresponds to a Kronecker product

$$U_4 = \mathbb{1}_N \otimes U_y \quad (46)$$

of an  $N$ -dimensional unit matrix  $\mathbb{1}_N$  for the states  $|\varphi_n\rangle$  and

$$U_y = \frac{1}{\sqrt{2}} \begin{pmatrix} 1 & 1 \\ -i & i \end{pmatrix} \quad (47)$$

for  $|g_{\pm}\rangle$ . Based on Eq. (32),  $U_y$  was chosen to fulfill

$$\frac{E_{Z,g}^0}{2} U_y^\dagger \begin{pmatrix} 0 & i \\ -i & 0 \end{pmatrix} U_y = \frac{E_{Z,g}^0}{2} \begin{pmatrix} 1 & 0 \\ 0 & -1 \end{pmatrix}. \quad (48)$$

We note, however, that the resulting Zeeman splitting between states  $|n_+\rangle$  and  $|n_-\rangle$  in  $H_N^a$  is not simply  $E_{Z,g}^0$  and changes with  $n$ . In contrast, the orbital level spacing is always  $\hbar\omega_g'$ . The remaining terms of the Hamiltonian are summarized in

$$H_N^b = U_4^\dagger H_N U_4 - H_N^a. \quad (49)$$

#### Step 5

We perturbatively decouple the two lowest QD states  $|0_{\pm}\rangle$  from higher states via a second-order SW transformation. The large energy is now provided by the level spacing  $\hbar\omega_g'$  in  $H_N^a$ , and  $H_N^b$  corresponds to the perturbation. The resulting projection ( $P_q^0$ ) onto the qubit subspace  $\Sigma_q = \{0_+, 0_-\}$  reads

$$H_q' = P_q^0 U_5^\dagger (H_N^a + H_N^b) U_5 P_q^0, \quad (50)$$

where the SW transformation is denoted by  $U_5$ . Neglecting global shifts in energy, the result can be written in terms of Pauli matrices,

$$H_q' = c_x \sigma'_x + c_y \sigma'_y + c_z \sigma'_z. \quad (51)$$

For the setup under study and with the standard representation in the basis  $\Sigma_q$ ,

$$\sigma'_x = \begin{pmatrix} 0 & 1 \\ 1 & 0 \end{pmatrix}, \quad \sigma'_y = \begin{pmatrix} 0 & -i \\ i & 0 \end{pmatrix}, \quad \sigma'_z = \begin{pmatrix} 1 & 0 \\ 0 & -1 \end{pmatrix}, \quad (52)$$

we find  $c_x = 0$  and  $c_y \propto E_z$  for arbitrarily large  $N$ . That is,  $c_z$  provides the Zeeman splitting between the qubit states, whereas  $c_y$  corresponds to the transverse coupling driven by  $E_z$ . In fact, within the second-order perturbation theory,  $c_y$  is fully determined by the coupling between states  $|0_{\pm}\rangle$  and  $|1_{\pm}\rangle$ , so that the result for  $c_y$  does not change for  $N > 2$ . This is different for  $c_z$ . The reason, in particular, is that  $H_g'$  features terms of type  $\sigma_{x,y}$  that couple the two spin blocks ( $\sigma_i$ : Pauli operators acting on the spin index  $\{+, -\}$  [1]). Because of

$$|\langle n_{\pm} | \sigma_{x,y} | m_{\mp} \rangle| \neq \delta_{mn}, \quad (53)$$

these also generate nonzero matrix elements between  $|0_{\pm}\rangle$  and  $|n_{\mp}\rangle$  with large  $n$ . However, as  $H_g'$  contains terms up to the second power in  $k_z$  only, the dominant contributions to  $c_z$  are provided within the subspace of states  $|0_{\pm}\rangle$ ,  $|1_{\pm}\rangle$ , and  $|2_{\pm}\rangle$ . Remarkably, we find from Taylor expansions that linear terms in  $B_y$  are due to the first four states  $|0_{\pm}\rangle$  and  $|1_{\pm}\rangle$  only. Hence, the calculated  $g$  factor  $g \equiv 2c_z/(\mu_B B_y)$  remains unchanged for  $N > 2$  (as for  $c_y$ ), provided that  $B_y$  is weak enough for the linear expansion of  $c_z$  to apply. In the main text, we use  $N = 3$  for all plots presenting the effective model. The quantitative corrections from  $N > 3$  to the Zeeman splitting are only expected in the regime where both  $E_y$  and  $B_y$  are large.

The full formulas for  $c_y$  and  $c_z$  are too lengthy to be displayed here. However, as mentioned above, we can perform a linear expansion in  $B_y$  when the Zeeman splitting is small compared to the orbital level spacing. The results are shown in Eqs. (A.1) and (A.2) of the Appendix, and we note that the corrections for both  $c_y$  and  $c_z$  are of order  $B_y^3$ . By keeping only the dominant terms, these formulas can be simplified even further. In particular, we find that  $\text{DRSOI} \gg \text{RSOI}$  in typical Ge/Si NW QDs, and conventional RSOI may therefore be neglected. The simplified results without RSOI are summarized in Eqs. (A.5) and (A.6).

### Step 6

From  $H'_q$ , Eq. (51), the final form of the effective  $2 \times 2$  Hamiltonian  $H_q$ , Eq. (13), is obtained through a unitary transformation

$$H''_q = U_6^\dagger H'_q U_6 = \frac{E_Z}{2} \sigma'_z + T_q \sigma'_x, \quad (54)$$

where  $E_Z$  is the Zeeman splitting and  $T_q = \bar{\nu} E_Z$  is the transverse coupling due to the electric field  $E_z$ . We recall that  $T_q = \nu_e \cos(\omega_{ac} t)$  for EDSR and  $T_q = \nu_c (a^\dagger + a)$  for operations based on the cavity field, with  $\nu_{e,c} = \bar{\nu} E_{z,0}^{e,c}$  as the coupling strengths. When  $U_6$  is chosen such that  $E_Z$  and  $\bar{\nu}$  are both positive, one identifies

$$E_Z = |2c_z|, \quad (55)$$

$$\bar{\nu} = \frac{|c_y(E_{z,0})|}{E_{z,0}}, \quad (56)$$

where  $E_{z,0}$  stands for an arbitrary electric field amplitude and  $c_y = c_y(E_z)$  is the transverse coupling coefficient derived in this section. Because the ac fields along the NW are small in the studied setup, corrections of type  $E_z^2$  in  $c_z$  [see, e.g., Eq. (A.2)] are neglected in Eq. (55), and, thus, the Zeeman splitting  $E_Z$  is independent of  $\cos(\omega_{ac} t)$  and  $(a^\dagger + a)$ , respectively.

We note that  $H_q$  is obtained from the formally equivalent  $H''_q$  when the Pauli operators  $\sigma'_i$  are replaced by  $\tilde{\sigma}_i$ , i.e., when the basis states  $|0_\pm\rangle$  in  $\Sigma_q$  are replaced by the corresponding eigenstates of  $H$  that form the qubit.

### Remarks

The unitary transformations presented here illustrate that the true basis states of the qubit will differ from  $|0_\pm\rangle$ , Eq. (34). The eigenstates may be calculated either by an inverse transformation or numerically, see Sec. III. However, we emphasize that knowledge of the qubit states is not required for the implementation of quantum gates proposed here. EDSR only requires knowledge about the Zeeman splitting and the presence of an electric-field-induced transverse coupling. Moreover, long-range qubit-qubit interactions mediated by the cavity field are independent of the basis states of the individual qubits (see also Sec. V).

## III. QUANTUM DOT: NUMERICAL ANALYSIS

### Basis states

The Zeeman energy  $E_Z$  and the coupling parameter  $\bar{\nu}$  in QDs with  $l_q \gg R$ , for which  $H$  of Eq. (5) applies, can also be calculated numerically. For this, we represent  $H = H(E_z)$  by a matrix with  $4N'$  basis states. The basis of the matrix reads  $\Sigma_{N'} = \{\Sigma_{N'}^g, \Sigma_{N'}^e\}$ , where

$$\Sigma_{N'}^{g,e} = \{0_+^{g,e}, 0_-^{g,e}, \dots, (N' - 1)_+^{g,e}, (N' - 1)_-^{g,e}\}, \quad (57)$$

and we denote the projector for  $\Sigma_{N'}$  by  $P_{N'}$ . The basis states are defined as

$$|n_\pm^g\rangle = |g_\pm\rangle \otimes |\varphi_n^g\rangle, \quad (58)$$

$$|n_\pm^e\rangle = |e_\pm\rangle \otimes |\varphi_n^e\rangle. \quad (59)$$

Here, analogous to Sec. II, the  $|\varphi_n^{g,e}\rangle$  are the eigenstates of the 1D harmonic oscillator

$$\left( \frac{\hbar^2 k_z^2}{2m_{g,e}} + V(z) \right) |\varphi_n^{g,e}\rangle = \hbar\omega_{g,e} \left( n + \frac{1}{2} \right) |\varphi_n^{g,e}\rangle, \quad (60)$$

where  $n$  is the quantum number and  $\omega_e = \omega_g \sqrt{m_g/m_e}$ . When an electric field  $E_z$  with amplitude  $E_{z,0}$  is applied along the NW, two approaches are suitable for the numerical calculation of  $E_Z$  and  $\bar{\nu}$  in  $H_q$ , Eq. (13). Provided that  $N'$  is chosen large enough, both approaches make use of an exact diagonalization in the degrees of freedom of the longitudinal coordinate  $z$ . However, they differ in the range of allowed  $E_{z,0}$  and in the computation time. Both algorithms are outlined below.

### Algorithm 1

The first approach requires calculation of all  $4N'$  eigenstates. As explained in more detail in the next paragraph, it applies for any strength of  $E_z$  and can therefore be regarded as generally valid. At first, we calculate all the eigenstates  $|m\rangle$  and corresponding eigenenergies  $E_m$  of  $P_{N'} H(0) P_{N'}$ . Based on this eigensystem, where  $m \in \{0, 1, \dots, 4N' - 1\}$  and  $E_0 \leq E_1 \leq \dots \leq E_{4N'-1}$ , we generate a transformation matrix  $U_0$  that diagonalizes the Hamiltonian according to

$$\text{diag}(E_0, E_1, \dots, E_{4N'-1}) = U_0^\dagger P_{N'} H(0) P_{N'} U_0. \quad (61)$$

The transverse coupling  $\nu \equiv \bar{\nu} E_{z,0}$  is then calculated via

$$\nu = |\langle 1 | U_0^\dagger P_{N'} H(E_{z,0}) P_{N'} U_0 | 0 \rangle|, \quad (62)$$

and the Zeeman energy  $E_Z$  is obtained through

$$E_Z = |\langle 1 | U_0^\dagger P_{N'} H(E_{z,0}) P_{N'} U_0 | 1 \rangle - \langle 0 | U_0^\dagger P_{N'} H(E_{z,0}) P_{N'} U_0 | 0 \rangle|. \quad (63)$$

We note that, for realistic  $E_{z,0}$ , the latter is very well approximated by  $E_1 - E_0$ , which is the Zeeman splitting between the qubit states in the absence of  $E_z$ .

When  $E_{z,0}$  is large, the two eigenstates of  $H(E_{z,0})$  with lowest energy cannot be expressed in terms of  $|0\rangle$  and  $|1\rangle$  only. In systems driven through EDSR, however, where  $E_z$  is an ac field that is in (quasi-)resonance with the Zeeman splitting  $E_1 - E_0$ , the dynamics are determined by the coupling strength induced between  $|0\rangle$  and  $|1\rangle$ , Eq. (62). Therefore, this algorithm applies for any strength of  $E_z$  when  $N'$  is large enough for the diagonalization in the degrees of freedom of the coordinate  $z$  to be accurate.

### Algorithm 2

The second approach applies for small  $E_{z,0}$  only and allows for reduced computation times when  $N'$  is chosen very large, because only four instead of  $4N'$  eigenstates need to be calculated and a transformation matrix  $U_0$  is not required. Analogously to the first method, we calculate the eigenenergies  $E_m$  of  $P_{N'}H(0)P_{N'}$  and the two eigenstates  $|0\rangle$  and  $|1\rangle$  of lowest energy. In addition, we compute the eigenenergies  $E'_m$  and the eigenstates  $|0'\rangle$  and  $|1'\rangle$  of  $P_{N'}H(E_{z,0})P_{N'}$ . When  $E_{z,0}$  is small, such that  $|0'\rangle \approx |0\rangle$ ,  $|1'\rangle \approx |1\rangle$ , and

$$|\langle 0|0'\rangle|^2 + |\langle 1|0'\rangle|^2 \simeq 1, \quad (64)$$

$$|\langle 0|1'\rangle|^2 + |\langle 1|1'\rangle|^2 \simeq 1, \quad (65)$$

one finds

$$\nu = \frac{E'_1 - E'_0}{2} |\langle 1|1'\rangle \langle 1'|0\rangle - \langle 1|0'\rangle \langle 0'|0\rangle|, \quad (66)$$

$$E_Z = (E'_1 - E'_0) (|\langle 0|0'\rangle|^2 + |\langle 1|1'\rangle|^2 - 1). \quad (67)$$

### Remarks

The plots in the main text were generated with the first, more general method, using  $N' = 10$ . The latter was chosen because, on the one hand,  $N' = 10$  is large enough so that notable changes in the results are not observed as  $N'$  is increased, and, on the other hand, it is small enough to enable fast evaluation, as  $40 \times 40$  matrices can be diagonalized quickly. For the Ge/Si NW QD considered in the main text, we find that plots from approaches 1 and 2 are basically indistinguishable at  $E_{z,0} \lesssim 2 \times 10^3$  V/m, i.e., for  $eE_{z,0}l_g/(\sqrt{2}\hbar\omega_g) \lesssim 0.1$  [see also Eq. (71)]. At  $E_{z,0} > 2 \times 10^3$  V/m, the  $\nu$  from method 2 become smaller than those from method 1. This deviation is expected, because the assumptions of approach 2 are no longer well fulfilled when  $E_{z,0}$  is large.

## IV. PARAMETER RANGE AND VALIDITY OF RESULTS

### Effective 1D Hamiltonian

In the presence of a Si shell, we estimate that the effective 1D Hamiltonian

$$H_{1D} = H_{LK} + H_{BP} + H_B + H_{DR} + H_{R,y} + H_{R,z} \quad (68)$$

is valid for  $2 \text{ nm} \lesssim R \lesssim 12 \text{ nm}$ . At  $R \lesssim 2 \text{ nm}$ , the holes notably leak into the Si shell, despite the large VB offset  $\sim 0.5 \text{ eV}$  [4] at the interface. Furthermore, the LK Hamiltonian loses validity when the cross section consists of very few atoms only [5, 6]. When both  $R$  and  $\gamma$  are large, a simple projection of the BP Hamiltonian onto the low-energy subspace is no longer reliable as the strain-induced coupling to higher bands may exceed the energy separation  $\propto R^{-2}$  [1].

In general,  $H_{1D}$  is valid as long as the low-energy  $4 \times 4$  subspace is well isolated from these higher bands. This criterion puts restrictions on the strength of  $E_y$  in our model, and the limits for  $E_y$  depend on the energy difference to the next excited band ( $|F_z| = 3/2$ ). Because the total angular momentum  $F_z$  along the Ge/Si NW is conserved in the spherical approximation, which applies well for both the LK and the BP Hamiltonian of the system, the hole spectrum can be calculated exactly in the absence of external fields, as outlined in Ref. [1]. Based on these exact spectra, we estimate that the  $4 \times 4$  subspace can be considered well isolated when

$$|E_y| \lesssim 5 \frac{\text{kV nm}^3}{\mu\text{m } R^3}. \quad (69)$$

This criterion holds for any shell thickness, and higher transverse subbands should be included when  $|E_y|$  is much larger than the boundary value. The proportionality to  $R^{-3}$  is consistent with  $U \propto R$  and the  $R^{-2}$ -type decrease of the level spacings. For  $R = 7.5 \text{ nm}$  discussed in the main text, Eq. (69) yields  $|E_y| \lesssim 12 \text{ V}/\mu\text{m}$ .

### Qubit Hamiltonian $H_q$

Our numerical and analytical results for  $H_q$  describing the qubit are based on the Hamiltonian  $H$ , Eq. (5). The latter is valid when both  $l_g \gg R$  and  $H_{1D}$  apply.

The perturbative approach from Sec. II furthermore assumes that  $m'_g$  in Eq. (27) is positive and finite, which corresponds to

$$\frac{2m_g\tilde{C}^2}{\hbar^2\Delta'} \ll 1. \quad (70)$$

In addition, the two SW transformations require that the block-off-diagonal terms are small enough for the perturbative decoupling to be possible. From careful analysis of all matrices, we deduce a list of inequalities that have to be fulfilled. It turns out, however, that all these criteria are usually very well met when Eq. (70) holds and when  $B_y$  is chosen such that the Zeeman splitting does not exceed the orbital level spacing. We note that the left-hand side of Eq. (70) roughly scales with  $R^{-2}$ . Based on all criteria, we find that the perturbative approach applies when  $5 \text{ nm} \lesssim R \lesssim 12 \text{ nm}$  for typical Ge/Si NW QDs, and the agreement between numerics (Sec. III) and the derived formulas improves as  $R$  increases. For small core radii  $R \lesssim 5 \text{ nm}$ , the Hamiltonian  $H_q$  should, e.g., be calculated numerically as described in Sec. III. The condition for the electric field amplitude  $E_{z,0}$  along the NW reads

$$E_{z,0} \ll \frac{\sqrt{2}\hbar\omega'_g}{l'_ge}. \quad (71)$$

This inequality has a simple physical meaning. For the perturbation theory to be applicable, the shift of the minimum of  $V(z)$  due to  $E_{z,0}$  should not exceed the confinement length  $l'_g$ . With  $m'_g \sim m_g$  and the value from Table I, one obtains

$E_{z,0} \ll 2.5 \text{ V nm}^2/l_g^3$ . For  $l_g = 50 \text{ nm}$  discussed in the main text, this implies  $E_{z,0} \ll 2 \times 10^4 \text{ V/m}$ .

The numerical results from Sec. III hold whenever  $H$  applies, provided that  $N'$  is large enough. Furthermore, they can provide detailed information about the basis states of the qubit, if required.

### Remarks

In conclusion, although the parameter range is limited due to the complexity of the system, our theories are very well suited for commonly used Ge/Si NWs and NW QDs [4, 7–16]. All electric fields considered in the main text are far below the boundary values listed here.

## V. CAVITY-BASED INTERACTIONS

### Electric cavity field

We consider a 1D superconducting transmission line resonator [17, 18] of length  $L_c$  along the  $x$  axis. The center conductor ranges from  $x = 0$  to  $x = L_c$ , and the distance between the ground planes and the center conductor is denoted by  $d$ . When  $c$  ( $l$ ) stands for the capacitance (inductance) per unit length of the resonator, the electric field  $E_c(x)$  within the cavity reads

$$E_c(x) = \frac{1}{d} \sum_{p=1}^{\infty} \sqrt{\frac{\hbar\omega_p}{cL_c}} \cos\left(\frac{p\pi x}{L_c}\right) (a_p^\dagger + a_p), \quad (72)$$

where

$$\hbar\omega_p = \frac{\hbar p\pi}{L_c \sqrt{lc}} \quad (73)$$

are the energies of the photon modes  $p \in \{1, 2, \dots\}$  inside the cavity. Details of the derivation can be found in Ref. [17]. In Eq. (72), the operators  $a_p^\dagger$  and  $a_p$  are the creation and annihilation operators, respectively, for the modes  $p$ , and obey the commutation relations  $[a_p, a_{p'}^\dagger] = a_p a_{p'}^\dagger - a_{p'}^\dagger a_p = \delta_{pp'}$  and  $[a_p, a_{p'}] = 0 = [a_p^\dagger, a_{p'}^\dagger]$ . With these ladder operators, the cavity photon Hamiltonian is

$$H_\gamma = \sum_{p=1}^{\infty} \hbar\omega_p \left( a_p^\dagger a_p + \frac{1}{2} \right). \quad (74)$$

In the hybrid system with Ge/Si NW QDs inside the cavity, we assume that the qubits are quasi-resonant with one particular photon mode  $p = \tilde{p}$  (typically  $\tilde{p} = 1, 2$ ), so that all other modes can be neglected. With the notation  $a \equiv a_{\tilde{p}}$ ,  $a^\dagger \equiv a_{\tilde{p}}^\dagger$ , and  $\omega_c \equiv \omega_{\tilde{p}}$ , the cavity electric field that is relevant for the qubit dynamics reduces to

$$E_c(x) = \frac{1}{d} \sqrt{\frac{\hbar\omega_c}{cL_c}} \cos\left(\frac{\tilde{p}\pi x}{L_c}\right) (a^\dagger + a), \quad (75)$$

and the relevant part of  $H_\gamma$  reads

$$H_\gamma = \hbar\omega_c a^\dagger a. \quad (76)$$

When a NW QD is located near an antinode of  $E_c(x)$ , with the cavity field oriented along the symmetry axis of the NW ( $z$  axis), the cavity-induced electric field inside the dot is

$$E_z = E_{z,0}^c (a^\dagger + a), \quad (77)$$

where the effective strength  $E_{z,0}^c$  corresponds to

$$E_{z,0}^c = \frac{1}{\epsilon_r d} \sqrt{\frac{\hbar\omega_c}{cL_c}}. \quad (78)$$

Because the hole states in Ge/Si NWs are located in the Ge core, the electric field  $E_z$  inside the NW QD is reduced compared to  $E_c$  by the relative permittivity  $\epsilon_r \simeq 16$  of Ge.

From a rough estimate, we obtain  $1/\sqrt{lc} \approx c_0/n_{\text{eff}}$  and  $E_{z,0}^c \propto \hbar\omega_c/\sqrt{\tilde{p}hd}$ , where  $c_0$  is the speed of light in vacuum,  $n_{\text{eff}}$  is the effective refractive index within the cavity, and  $h$  is the height of the superconductor. This relation allows us to estimate experimentally feasible values of  $E_{z,0}^c$ . Based on the numbers provided in Refs. [17–19], we consider  $\hbar\omega_c = 25 \mu\text{eV}$ ,  $d = 5 \mu\text{m}$ ,  $h = 0.2 \mu\text{m}$ ,  $\tilde{p} = 2$ , and  $\epsilon_r E_{z,0}^c = 0.2 \text{ V/m}$  as reference values. When  $hd = 1 \mu\text{m}^2$  is reduced to  $hd = 10^{-2} \mu\text{m}^2$ , which seems feasible, one obtains  $E_{z,0}^c = 0.7 \text{ V/m}$  for  $\tilde{p} = 1$  and  $\hbar\omega_c = 0.1 \text{ meV}$ . In the main text, we therefore set  $E_{z,0}^c = 3 \text{ V/m}$  for the example of  $\hbar\omega_c \simeq 0.35 \text{ meV}$ . Higher values for  $E_{z,0}^c$  can easily be realized for qubits with larger Zeeman energies, but may also be possible for fixed frequencies when the fabrication can be further optimized (reducing the cavity mode volume).

Finally, we note that magnetic fields  $|B_y| > 0.2 \text{ T}$  imply that the superconducting transmission line resonators are fabricated from suitable materials, as  $B_y$  exceeds the critical magnetic field of commonly used Nb resonators [18–20]. One possible material is NbTiN, which remains superconducting at magnetic fields of several Tesla [21, 22].

### Qubit-cavity coupling

The coupled system of cavity field and qubit is described by  $H_{c-q} = H_q + H_\gamma$ ,

$$H_{c-q} = \frac{E_Z}{2} \tilde{\sigma}_z + \nu_c \tilde{\sigma}_x (a^\dagger + a) + \hbar\omega_c a^\dagger a, \quad (79)$$

where we recall the notation  $\nu_c = \bar{\nu} E_{z,0}^c$ . Introducing

$$\tilde{\sigma}_\pm = \tilde{\sigma}_x \pm i\tilde{\sigma}_y \quad (80)$$

as the raising and lowering operator, respectively, of the qubit, one obtains

$$H_{c-q} = \frac{E_Z}{2} \tilde{\sigma}_z + \frac{\nu_c}{2} (\tilde{\sigma}_+ + \tilde{\sigma}_-) (a^\dagger + a) + \hbar\omega_c a^\dagger a. \quad (81)$$

When the detuning

$$\Delta_q \equiv E_Z - \hbar\omega_c \quad (82)$$

between the qubit and the cavity is small, i.e.,  $|\Delta_q| \ll E_Z$  and  $|\Delta_q| \ll \hbar\omega_c$ , one can adopt the rotating wave approximation [23] and get the Jaynes-Cummings Hamiltonian

$$H_{c-q} = \frac{E_Z}{2} \tilde{\sigma}_z + \frac{\nu_c}{2} (\tilde{\sigma}_+ a + \tilde{\sigma}_- a^\dagger) + \hbar\omega_c a^\dagger a. \quad (83)$$

If, for instance, the qubit is prepared in the excited state,  $H_{c-q}$  implies that the excitation is coherently swapped between the qubit and the cavity. At resonance and at low temperatures ( $k_B T \ll \hbar\omega_c$ ;  $k_B$  is the Boltzmann constant,  $T$  the temperature), for which the occupation number of the cavity mode approaches zero, the resulting Rabi oscillation has a full-cycle duration on the order of  $\pi\hbar/\nu_c$ .

### Qubit-qubit coupling

Long-distance two-qubit gates can be implemented by operating two qubits near resonance with the cavity field. With the index in superscript parentheses labeling qubits, the corresponding Hamiltonian reads

$$H_{c-2q} = \sum_{i=1}^2 \left[ \frac{E_Z^{(i)}}{2} \tilde{\sigma}_z^{(i)} + \frac{\nu_c^{(i)}}{2} (\tilde{\sigma}_+^{(i)} a + \tilde{\sigma}_-^{(i)} a^\dagger) \right] + \hbar\omega_c a^\dagger a. \quad (84)$$

Analogous to the single-qubit case, this Hamiltonian applies for  $|\Delta_q^{(i)}| \ll E_Z^{(i)}$  and  $|\Delta_q^{(i)}| \ll \hbar\omega_c$ , where  $\Delta_q^{(i)} = E_Z^{(i)} - \hbar\omega_c$ . If furthermore  $\nu_c^{(i)} \ll |\Delta_q^{(i)}|$ , it is possible to remove the qubit-cavity interaction

$$H_{c-2q}^{\text{int}} = \sum_{i=1}^2 \frac{\nu_c^{(i)}}{2} (\tilde{\sigma}_+^{(i)} a + \tilde{\sigma}_-^{(i)} a^\dagger) \quad (85)$$

perturbatively via a Schrieffer-Wolff transformation [17, 23–25]. For this, we define

$$\tilde{H}_{c-2q} = e^T H_{c-2q} e^{-T}, \quad (86)$$

where  $H_{c-2q} = H_{c-2q}^0 + H_{c-2q}^{\text{int}}$  and  $T = T_1 + \mathcal{O}(\nu_c^3/\Delta_q^3)$  with

$$T_1 = \sum_{i=1}^2 \frac{\nu_c^{(i)}}{2\Delta_q^{(i)}} (\tilde{\sigma}_+^{(i)} a - \tilde{\sigma}_-^{(i)} a^\dagger). \quad (87)$$

Exploiting  $[T_1, H_{c-2q}^0] = -H_{c-2q}^{\text{int}}$ , expansion of Eq. (86) yields

$$\begin{aligned} \tilde{H}_{c-2q} &= H_{c-2q}^0 + \frac{1}{2} [T_1, H_{c-2q}^{\text{int}}] + \mathcal{O}\left(\frac{\nu_c^4}{\Delta_q^3}\right) \\ &= H_{c-2q}^0 + \sum_{i=1}^2 \frac{(\nu_c^{(i)})^2}{2\Delta_q^{(i)}} (1 + \tilde{\sigma}_z^{(i)} + 2\tilde{\sigma}_z^{(i)} a^\dagger a) \\ &\quad + \frac{J_{xy}}{8} (\tilde{\sigma}_+^{(1)} \tilde{\sigma}_-^{(2)} + \tilde{\sigma}_-^{(1)} \tilde{\sigma}_+^{(2)}) + \mathcal{O}\left(\frac{\nu_c^4}{\Delta_q^3}\right), \end{aligned} \quad (88)$$

where we defined

$$J_{xy} = J_{xy}^{(1,2)} = \nu_c^{(1)} \nu_c^{(2)} \left( \frac{1}{\Delta_q^{(1)}} + \frac{1}{\Delta_q^{(2)}} \right). \quad (89)$$

The subscript of  $J_{xy}$  indicates that the qubit-qubit interaction in  $\tilde{H}_{c-2q}$  is equivalent to a transverse spin-spin coupling,

$$\tilde{\sigma}_+^{(1)} \tilde{\sigma}_-^{(2)} + \tilde{\sigma}_-^{(1)} \tilde{\sigma}_+^{(2)} = 2 (\tilde{\sigma}_x^{(1)} \tilde{\sigma}_x^{(2)} + \tilde{\sigma}_y^{(1)} \tilde{\sigma}_y^{(2)}). \quad (90)$$

Finally, when the photon number operator in Eq. (88) is replaced by the average occupation number, i.e.,  $a^\dagger a \rightarrow \langle a^\dagger a \rangle \equiv \bar{n}$ , and when global shifts in energy are neglected,  $\tilde{H}_{c-2q}$  results in the effective two-qubit Hamiltonian

$$H_{q-q} = \sum_{i=1}^2 \frac{\bar{E}_Z^{(i)}}{2} \tilde{\sigma}_z^{(i)} + \frac{J_{xy}}{8} (\tilde{\sigma}_+^{(1)} \tilde{\sigma}_-^{(2)} + \tilde{\sigma}_-^{(1)} \tilde{\sigma}_+^{(2)}), \quad (91)$$

where

$$\bar{E}_Z^{(i)} = E_Z^{(i)} + (1 + 2\bar{n}) \frac{(\nu_c^{(i)})^2}{\Delta_q^{(i)}}. \quad (92)$$

The cavity-induced correction to the Zeeman splitting that is independent of (proportional to)  $\bar{n}$  corresponds to the Lamb shift (ac Stark shift) [17, 23].

### Two-qubit gates

The Hamiltonian  $H_{q-q}$ , Eq. (91), enables the implementation of entangling two-qubit gates ( $i$ SWAP,  $\sqrt{i}$ SWAP) and, thus, in combination with single-qubit operations, allows for universal quantum computing [17, 23–26]. For illustration purposes, we discuss below the special case  $\bar{E}_Z^{(1)} = \bar{E}_Z^{(2)} \equiv \bar{E}_Z$  in more detail. In the basis  $\Sigma_{q-q} = \{|11\rangle, |10\rangle, |01\rangle, |00\rangle\}$  with  $|ab\rangle = |a^{(1)}\rangle \otimes |b^{(2)}\rangle$ , where the qubit states  $|0\rangle$  (ground) and  $|1\rangle$  (excited) are eigenstates of  $\tilde{\sigma}_z$  with eigenvalues  $\mp 1$ , the matrix representation of  $H_{q-q}$  is of the simple form

$$H_{q-q} = \begin{pmatrix} \bar{E}_Z & 0 & 0 & 0 \\ 0 & 0 & J_{xy}/2 & 0 \\ 0 & J_{xy}/2 & 0 & 0 \\ 0 & 0 & 0 & -\bar{E}_Z \end{pmatrix}. \quad (93)$$

The eigenstates and eigenenergies are  $|11\rangle$ ,  $(|10\rangle \pm |01\rangle)/\sqrt{2}$ ,  $|00\rangle$ , and  $\bar{E}_Z$ ,  $\pm J_{xy}/2$ ,  $-\bar{E}_Z$ , respectively. Provided that  $H_{q-q}$  is constant within the time interval  $0 \leq t' \leq t$ , one finds from the Schrödinger equation that the time evolution  $|\psi(t)\rangle = U_{xy}(t) |\psi(0)\rangle$  for an arbitrary state  $|\psi(0)\rangle$  is described by the operator

$$U_{xy}(t) = \begin{pmatrix} e^{-i\bar{E}_Z t/\hbar} & 0 & 0 & 0 \\ 0 & f_{xy}(t) & g_{xy}(t) & 0 \\ 0 & g_{xy}(t) & f_{xy}(t) & 0 \\ 0 & 0 & 0 & e^{i\bar{E}_Z t/\hbar} \end{pmatrix}, \quad (94)$$

where

$$f_{xy}(t) = \cos\left(\frac{J_{xy}t}{2\hbar}\right), \quad (95)$$

$$g_{xy}(t) = -i \sin\left(\frac{J_{xy}t}{2\hbar}\right). \quad (96)$$



We note that the relation  $U_{xy}(t_2)U_{xy}(t_1) = U_{xy}(t_1+t_2)$  may easily be verified. After the time  $t_{i\text{SWAP}} = \pi\hbar/|J_{xy}|$ , the states  $|10\rangle$  and  $|01\rangle$  have been coherently exchanged, which is commonly referred to as an  $i\text{SWAP}$  operation. For  $J_{xy} > 0$ ,

$$U_{xy}(t_{i\text{SWAP}}) = \begin{pmatrix} e^{-i\pi\bar{E}_Z/J_{xy}} & 0 & 0 & 0 \\ 0 & 0 & -i & 0 \\ 0 & -i & 0 & 0 \\ 0 & 0 & 0 & e^{i\pi\bar{E}_Z/J_{xy}} \end{pmatrix}, \quad (97)$$

and, for  $J_{xy} < 0$ ,

$$U_{xy}(t_{i\text{SWAP}}) = \begin{pmatrix} e^{i\pi\bar{E}_Z/J_{xy}} & 0 & 0 & 0 \\ 0 & 0 & i & 0 \\ 0 & i & 0 & 0 \\ 0 & 0 & 0 & e^{-i\pi\bar{E}_Z/J_{xy}} \end{pmatrix}. \quad (98)$$

An entangling  $\sqrt{i\text{SWAP}}$  gate is obtained when the system evolves for the time  $t_{i\text{SWAP}}/2$ . We note that also  $i\text{SWAP}$  is entangling, in stark contrast to the SWAP operation that we recall below.

For comparison, we consider the Hamiltonian for an isotropic (Heisenberg-type) spin-spin coupling

$$H_{q-q}^H = \sum_{i=1}^2 \frac{E_Z}{2} \tilde{\sigma}_z^{(i)} + \frac{J_H}{4} \tilde{\sigma}^{(1)} \cdot \tilde{\sigma}^{(2)} - \frac{J_H}{4}, \quad (99)$$

where  $\tilde{\sigma} = (\tilde{\sigma}_x, \tilde{\sigma}_y, \tilde{\sigma}_z)$  is the vector of Pauli matrices and the global energy shift  $-J_H/4$  was added for convenience. In matrix form, with basis  $\Sigma_{q-q}$  as above,  $H_{q-q}^H$  reads

$$H_{q-q}^H = \begin{pmatrix} E_Z & 0 & 0 & 0 \\ 0 & -J_H/2 & J_H/2 & 0 \\ 0 & J_H/2 & -J_H/2 & 0 \\ 0 & 0 & 0 & -E_Z \end{pmatrix}. \quad (100)$$

The resulting time evolution  $|\psi(t)\rangle = U_H(t)|\psi(0)\rangle$  for an arbitrary state  $|\psi(0)\rangle$  is given by

$$U_H(t) = \begin{pmatrix} e^{-iE_Z t/\hbar} & 0 & 0 & 0 \\ 0 & f_H(t) & g_H(t) & 0 \\ 0 & g_H(t) & f_H(t) & 0 \\ 0 & 0 & 0 & e^{iE_Z t/\hbar} \end{pmatrix}, \quad (101)$$

where

$$f_H(t) = \frac{1}{2} \left( 1 + e^{iJ_H t/\hbar} \right), \quad (102)$$

$$g_H(t) = \frac{1}{2} \left( 1 - e^{iJ_H t/\hbar} \right). \quad (103)$$

The operation time for a SWAP gate is  $t_{\text{SWAP}} = \pi\hbar/|J_H|$  (usually  $J_H > 0$ ),

$$U_H(t_{\text{SWAP}}) = \begin{pmatrix} e^{-i\pi E_Z/|J_H|} & 0 & 0 & 0 \\ 0 & 0 & 1 & 0 \\ 0 & 1 & 0 & 0 \\ 0 & 0 & 0 & e^{i\pi E_Z/|J_H|} \end{pmatrix}, \quad (104)$$

and the entangling  $\sqrt{\text{SWAP}}$  operation [27] is realized after the time  $t_{\text{SWAP}}/2$ . As for  $U_{xy}$ , we note that verification of  $U_H(t_2)U_H(t_1) = U_H(t_1+t_2)$  is easily possible for  $U_H$ , which implies  $(\sqrt{\text{SWAP}})^2 = \text{SWAP}$  (analogous for  $i\text{SWAP}$ ).

## VI. CHARGE NOISE

### Perturbation due to electric field fluctuations

The Hamiltonian  $H_q$ , Eq. (13), depends on the applied electric fields, and random fluctuations  $\delta E_y(t)$  and  $\delta E_z(t)$  therefore lead to a noisy perturbation

$$\delta H_q^{\text{el}}(t) = \frac{\delta E_Z(t)}{2} \tilde{\sigma}_z + \delta T_q(t) \tilde{\sigma}_x. \quad (105)$$

Linear expansion yields

$$\delta E_Z(t) \simeq (\partial_{E_y} E_Z) \delta E_y(t) + (\partial_{E_z} E_Z) \delta E_z(t), \quad (106)$$

$$\delta T_q(t) \simeq (\partial_{E_y} T_q) \delta E_y(t) + (\partial_{E_z} T_q) \delta E_z(t), \quad (107)$$

where the partial derivatives are evaluated at the electric fields  $E_y$  and  $E_z$  applied to the QD. This implies  $\delta E_Z(t) \simeq 0$  and  $\delta T_q(t) \simeq 0$  for an idle qubit, because all first derivatives vanish at  $E_y = 0 = E_z$ . That is, the proposed setup is highly insensitive to charge noise when the electric fields are switched off during the waiting time between quantum operations. The system, however, becomes sensitive to electrical noise when  $E_y$  is applied in order to induce the DRSOI. Since, as shown in the main text, single-qubit gates are much faster than two-qubit gates, the system performance is limited by the noisy perturbations during two-qubit operations, and below we study the resulting lifetimes in further detail.

### Relaxation and dephasing at maximal $\bar{\nu}$

The long-distance two-qubit gates are much slower than single-qubit gates. During two-qubit operations,  $E_y$  should therefore be chosen such that the coupling parameter  $\bar{\nu}$  is maximal, which implies  $\partial_{E_y} T_q = 0$ . Furthermore,  $\partial_{E_z} E_Z = 0$ , as illustrated, e.g., in Eq. (A.2). When the electric field fluctuations  $\delta E_\alpha(t)$ ,  $\alpha \in \{y, z\}$ , are related to the voltage fluctuations  $\delta V_\alpha(t)$  in the corresponding electric gates by  $\delta E_\alpha(t) = \kappa_\alpha \delta V_\alpha(t)$ , we find

$$\delta E_Z(t) \simeq \kappa_y (\partial_{E_y} E_Z) \delta V_y(t), \quad (108)$$

$$\delta T_q(t) \simeq \kappa_z \bar{\nu} \delta V_z(t), \quad (109)$$

where the  $\kappa_\alpha$  are device and geometry dependent constants. We recall that  $T_q = \bar{\nu} E_z$  and, thus,  $\partial_{E_z} T_q = \bar{\nu}$ , which is used in Eq. (109).

The relaxation ( $T_1^{\text{el}}$ ) and dephasing ( $T_\varphi^{\text{el}}$ ) times of the qubit in the presence of  $\delta H_q^{\text{el}}(t)$  can be calculated with the Bloch-Redfield theory [28–30]. With  $\omega_Z \equiv E_Z/\hbar$  and  $\text{Re}[\dots]$  as the real part, the rates read

$$\begin{aligned} \frac{1}{T_1^{\text{el}}} &= \frac{4}{\hbar^2} \int_0^\infty \cos(\omega_Z t) \text{Re}[\langle \delta T_q(0) \delta T_q(t) \rangle] dt \\ &= \frac{2}{\hbar^2} \int_{-\infty}^\infty \cos(\omega_Z t) \langle \delta T_q(0) \delta T_q(t) \rangle dt \end{aligned} \quad (110)$$

and

$$\begin{aligned} \frac{1}{T_\varphi^{\text{el}}} &= \frac{1}{\hbar^2} \int_0^\infty \text{Re}[\langle \delta E_Z(0) \delta E_Z(t) \rangle] dt \\ &= \frac{1}{2\hbar^2} \int_{-\infty}^\infty \langle \delta E_Z(0) \delta E_Z(t) \rangle dt. \end{aligned} \quad (111)$$

The correlation functions obtained from ensemble averages  $\langle \dots \rangle$  fulfill  $\langle \delta T_q(0) \delta T_q(-t) \rangle = \langle \delta T_q(0) \delta T_q(t) \rangle^*$  and  $\langle \delta E_Z(0) \delta E_Z(-t) \rangle = \langle \delta E_Z(0) \delta E_Z(t) \rangle^*$ , where the asterisk denotes complex conjugation, because the correlation functions are invariant under time translation and  $\delta T_q(t)$  and  $\delta E_Z(t)$  are hermitian. We note that the Bloch-Redfield approach requires  $\langle \delta E_Z(t) \rangle = 0 = \langle \delta T_q(t) \rangle$ , which is fulfilled for  $\langle \delta V_\alpha(t) \rangle = 0$  combined with Eqs. (108) and (109). When we introduce the spectral functions [31]

$$\begin{aligned} S_{V_\alpha}(\omega) &\equiv \int_{-\infty}^\infty e^{i\omega t} \langle \delta V_\alpha(t) \delta V_\alpha(0) \rangle dt \\ &= \int_{-\infty}^\infty e^{-i\omega t} \langle \delta V_\alpha(0) \delta V_\alpha(t) \rangle dt, \end{aligned} \quad (112)$$

i.e., the Fourier transforms of  $\langle \delta V_\alpha(t) \delta V_\alpha(0) \rangle = \langle \delta V_\alpha(0) \delta V_\alpha(-t) \rangle$ , Eqs. (110) and (111) take the form

$$\frac{1}{T_1^{\text{el}}} = \frac{\kappa_z^2 \bar{\nu}^2}{\hbar^2} [S_{V_z}(\omega_Z) + S_{V_z}(-\omega_Z)], \quad (113)$$

$$\frac{1}{T_\varphi^{\text{el}}} = \frac{\kappa_y^2}{2\hbar^2} (\partial_{E_y} E_Z)^2 S_{V_y}(0). \quad (114)$$

$S_{V_z}(\omega_Z)$  describes the process in which the gate for  $E_z$  absorbs the energy  $E_Z$  from the qubit, and vice versa for  $S_{V_z}(-\omega_Z)$  [31]. In contrast to the relaxation, dephasing happens without an energy transfer between the gate and the qubit, and it is correspondingly quantified by  $S_{V_y}(0)$ .

A major source of electrical noise is the Johnson-Nyquist noise [32, 33]. Following Refs. [31, 33], we therefore consider the spectral functions

$$S_{V_\alpha}(\omega) = \frac{2R_\alpha \hbar \omega}{1 - e^{-\beta_\alpha \hbar \omega}}, \quad (115)$$

where  $\beta_\alpha \equiv 1/(k_B T_\alpha)$  and  $R_\alpha$  ( $T_\alpha$ ) is the effective resistance (temperature) of the gate that generates  $E_\alpha$ . We note in passing that these spectral functions fulfill  $S_{V_\alpha}(\omega) = e^{\beta_\alpha \hbar \omega} S_{V_\alpha}(-\omega)$ , which corresponds to the detailed balance relation for a noise source in thermal equilibrium. Furthermore, the equality  $\langle \delta V_\alpha(0) \delta V_\alpha(-t) \rangle = \langle \delta V_\alpha(0) \delta V_\alpha(t) \rangle^*$  is ensured because  $S_{V_\alpha}(\omega)$  is real. Finally, substitution into Eqs. (113) and (114) yields

$$\frac{1}{T_1^{\text{el}}} = \frac{2\kappa_z^2 \bar{\nu}^2 R_z E_Z (e^{\beta_z E_Z} + 1)}{\hbar^2 (e^{\beta_z E_Z} - 1)}, \quad (116)$$

$$\frac{1}{T_\varphi^{\text{el}}} = \frac{\kappa_y^2}{\hbar^2} (\partial_{E_y} E_Z)^2 R_y k_B T_y. \quad (117)$$

The decoherence time  $T_2^{\text{el}}$  obeys the relation  $1/T_2^{\text{el}} = 1/(2T_1^{\text{el}}) + 1/T_\varphi^{\text{el}}$  [29, 30].

## Numerical estimates

For numerical estimates of the lifetimes discussed above, we set  $T_y = T_z \sim 10$  mK on the order of typical sample temperatures [18, 20]. When  $k_B T_z \ll E_Z$ , which is very well fulfilled for  $E_Z > 3$   $\mu\text{eV}$  here, the gates can only absorb energy and the relaxation rate becomes independent of the temperature,

$$\frac{1}{T_1^{\text{el}}} = \frac{2\kappa_z^2 \bar{\nu}^2 R_z E_Z}{\hbar^2}. \quad (118)$$

From an estimate based on typical gate dimensions (length  $\sim 1$  cm; cross section  $\sim 10^3$  nm<sup>2</sup>) and the residual resistivities of copper and gold ( $\sim 10^{-11}$   $\Omega\text{m}$ ), we choose  $R_y = R_z \sim 10^2$   $\Omega$ . Assuming that the material between the gates and the NW has a permittivity similar to that of Ge,  $\kappa_y$  can be approximated by  $\kappa_y \approx 1/d_y$ , where  $d_y \sim 0.1$   $\mu\text{m}$  is the distance between the electric gates for  $E_y$ . Because the NW QD is usually located above the gates that generate the confinement along the NW axis [20, 34–36], it is likely that the conversion factor for  $\delta E_z(t)$  is smaller than that for  $\delta E_y(t)$ , and we set here  $\kappa_z = 1/\mu\text{m} = \kappa_y/10$ . We emphasize, however, that both  $\kappa_y$  and  $\kappa_z$  depend strongly on the details of the setup.

The derivatives  $\partial_{E_y} E_Z$  and  $\partial_{E_z} T_q = \bar{\nu}$  are extracted from the numerical results summarized in Fig. 4 of the main text. At magnetic fields  $|B_y| \lesssim 0.5$  T,  $\bar{\nu}$  is maximal for  $E_y \simeq 1.8$  V/ $\mu\text{m}$ . At this electric field, we calculate  $\bar{\nu} \simeq 10|B_y|$  nm e/T, and find  $g \simeq 3.4$  and  $\partial_{E_y} g \simeq -1.6$   $\mu\text{m}/\text{V}$  for the  $g$  factor. With  $E_Z = |g\mu_B B_y|$ , substitution of all numbers into Eqs. (117) and (118) yields

$$T_\varphi^{\text{el}} \sim \frac{3.7 \times 10^{-2} \text{ s T}^2}{B_y^2}, \quad (119)$$

$$T_1^{\text{el}} \sim \frac{6.3 \times 10^{-7} \text{ s T}^3}{|B_y|^3}, \quad (120)$$

which, in terms of the Zeeman energy, is equivalent to

$$T_\varphi^{\text{el}} \sim \frac{1.4 \times 10^3 \text{ s } \mu\text{eV}^2}{E_Z^2}, \quad (121)$$

$$T_1^{\text{el}} \sim \frac{4.8 \text{ s } \mu\text{eV}^3}{E_Z^3}. \quad (122)$$

We note that  $T_\varphi^{\text{el}} \propto 1/E_Z^2$ , whereas  $T_1^{\text{el}} \propto 1/E_Z^3$ . Because the dephasing due to Johnson-Nyquist noise is strongly suppressed at low temperatures, we find here that  $T_1^{\text{el}} \ll T_\varphi^{\text{el}}$  for all reasonable  $B_y$ , leading to  $T_2^{\text{el}} = 2T_1^{\text{el}}$ .

In the example of a rather strong magnetic field  $B_y = 1.5$  T,  $\bar{\nu}$  peaks at  $E_y \simeq 1.1$  V/ $\mu\text{m}$ . At these fields, we obtain  $\bar{\nu} \simeq 16$  nm e,  $E_Z \simeq 0.35$  meV, and  $\partial_{E_y} E_Z \simeq -0.13$  nm e. The resulting lifetimes are  $T_\varphi^{\text{el}} \sim 19$  ms and  $T_1^{\text{el}} \sim 0.15$   $\mu\text{s}$ , and we mention in passing that these are very similar to the lifetimes extrapolated from Eqs. (119) to (122) derived for the case of relatively weak  $B_y$ . Again,  $T_2^{\text{el}} = 2T_1^{\text{el}}$ , i.e., the dephasing is negligible compared to the relaxation.

### Remarks

For both strong and weak magnetic fields, we find that the above calculated relaxation times are relatively close to the operation times of cavity-based two-qubit gates. In order to enhance the gate fidelities, relaxation due to Johnson-Nyquist noise should be suppressed by choosing a setup with small  $\kappa_z$ . For instance, when the details of the setup are designed such that  $\kappa_z = 0.1/\mu\text{m}$  instead of  $\kappa_z = 1/\mu\text{m}$  assumed above, the lifetimes  $T_1^{\text{el}}$  and  $T_2^{\text{el}}$  are prolonged by two orders of magnitude because of  $T_1^{\text{el}} \propto 1/\kappa_z^2$ . Further possibilities for increasing noise-limited gate fidelities are discussed in the main text.

We also note that high-frequency cut-offs were not considered in the analysis of the electrical noise. Consequently, the correlation functions  $\langle \delta T_q(0) \delta T_q(t) \rangle$  and  $\langle \delta E_Z(0) \delta E_Z(t) \rangle$  cannot be calculated explicitly as the spectral functions do not converge at infinite  $\omega$ , and, moreover, one finds  $T_1^{\text{el}} \rightarrow 0$  in the limit  $E_Z \rightarrow \infty$ . Cut-offs in the spectral functions of noisy perturbations can have various origins. When spin qubits relax via the phonon bath, for instance, the lifetimes turn out to be minimal when the corresponding phonon wavelength matches the dot size [23, 29, 37, 38]. This is because the relevant matrix elements vanish after integration over the wave functions when the phonon wavelength is much smaller than

the QD. Analogously, one may argue that  $T_1^{\text{el}}$  increases when  $E_Z \gtrsim \hbar\pi c_0 / (2l_g \sqrt{\epsilon_r}) \sim 1 \text{ eV}$ . Since the speed of light is by orders of magnitude greater than the speed of sound in Ge, this wavelength-based cut-off for charge noise occurs at much higher energies than that for phonons [38]. It is likely that other mechanisms in the metal itself lead to an increase of  $T_1^{\text{el}}$  and  $T_2^{\text{el}}$  at  $E_Z < 1 \text{ eV}$  already. However, we assume that high-frequency cut-offs in the spectral functions of the Johnson-Nyquist noise do not set in within the range of Zeeman energies discussed here. If they do occur, the resulting lifetimes will be increased significantly.

Finally, three more features of the proposed setup are worth mentioning in the context of charge noise. First, we note that the confinement length  $l_g$  presents an additional control parameter for the  $g$  factor [see, e.g., Eqs. (A.2) and (A.6)]. Hence, if required, fine tuning of  $l_g^{(i)}$  should allow realizing both  $\partial_{E_y^{(i)}} T_q^{(i)} = 0$  (maximal  $\bar{\nu}^{(i)}$ ) and the desired  $\Delta_q^{(i)}$  for any qubit  $i$  in the cavity. Second, static electric fields from the substrate, if present, will most likely be oriented along the  $y$  axis. Therefore, in order to achieve the desired  $E_y$  (particularly  $E_y = 0$ ), they may easily be compensated with the electric gates. Third, radial fields from the Ge/Si interface, if present, do not break the symmetry of the wire and may result in small corrections to  $\Delta$ ,  $C$ , and  $K$  only. All these properties are useful in an experimental realization.

### Appendix: RESULTS FROM EFFECTIVE MODEL

Below, we summarize the coefficients  $c_y$  and  $c_z$  of  $H'_q$ , Eq. (51), that result from the perturbative analysis described in Sec. II. Although the full results are lengthy and cannot be written out explicitly here, a Taylor expansion in the magnetic field  $B_y$  for  $N \rightarrow \infty$  yields

$$c_y = \mu_B B_y E_z \frac{2eC'}{(\hbar\omega'_g)^2} e^{-\left(\frac{C'}{l'_g \hbar\omega'_g}\right)^2} \left[ (K - (K + M) \sin^2 \theta) - \frac{L\tilde{C}}{l'^2_g \Delta'} \right] + \mathcal{O}(B_y^3) \quad (\text{A.1})$$

and

$$c_z = \mu_B B_y e^{-\left(\frac{C'}{l'_g \hbar\omega'_g}\right)^2} \left[ (K - (K + M) \sin^2 \theta) \left( 1 - \frac{C'^2 e^2 E_z^2}{(\hbar\omega'_g)^4} \right) - \frac{L\tilde{C}}{l'^2_g \Delta'} \right] + \mathcal{O}(B_y^3). \quad (\text{A.2})$$

The correction  $\propto E_z^2$  in  $c_z$  is negligible for the small electric fields  $E_z$  in our setup. In the regime of relatively weak  $B_y$ , where the linear expansion in  $B_y$  applies, the coefficients can therefore be summarized as follows,

$$c_y \simeq E_z \frac{2eC'}{(\hbar\omega'_g)^2} c_z, \quad (\text{A.3})$$

$$c_z \simeq \mu_B B_y e^{-\left(\frac{C'}{l'_g \hbar\omega'_g}\right)^2} \left[ (K - (K + M) \sin^2 \theta) - \frac{L\tilde{C}}{l'^2_g \Delta'} \right]. \quad (\text{A.4})$$

Finally, because the DRSOI is much stronger than the conventional RSOI [1], it turns out that the latter results in small quantitative corrections only and may be omitted. For  $\alpha \rightarrow 0$ , one finds  $\Delta' \rightarrow \tilde{\Delta}$ ,  $C' \rightarrow 2CeE_y U / \tilde{\Delta}$ ,  $\tilde{C} \rightarrow C\Delta / \tilde{\Delta}$ ,  $\omega'_g \rightarrow \tilde{\omega}_g$ ,  $l'_g \rightarrow \tilde{l}_g$ ,

and the coefficients read

$$c_y \simeq E_z \frac{4e^2 U C E_y}{(\hbar \tilde{\omega}_g)^2 \tilde{\Delta}} c_z, \quad (\text{A.5})$$

$$c_z \simeq \mu_B B_y e^{-\left(\frac{2e U C E_y}{l_g \hbar \tilde{\omega}_g \tilde{\Delta}}\right)^2} \left( \tilde{K} - \frac{L C \Delta}{\tilde{l}_g^2 \tilde{\Delta}^2} \right), \quad (\text{A.6})$$

where  $\tilde{l}_g = l_g \sqrt{\tilde{\omega}_g / \omega_g}$  and

$$\tilde{K} = K - \frac{(K + M) E_y^2}{\left(\frac{\tilde{\Delta} + \Delta}{2eU}\right)^2 + E_y^2}, \quad (\text{A.7})$$

$$\tilde{\Delta} = \sqrt{\Delta^2 + (2e E_y U)^2}, \quad (\text{A.8})$$

$$\tilde{\omega}_g = \omega_g \sqrt{1 - \frac{2m_g C^2 \Delta^2}{\hbar^2 \tilde{\Delta}^3}}. \quad (\text{A.9})$$

- 
- [1] C. Kloeffer, M. Trif, and D. Loss, Phys. Rev. B **84**, 195314 (2011).
- [2] R. Winkler, *Spin-Orbit Coupling Effects in Two-Dimensional Electron and Hole Systems* (Springer, Berlin, 2003).
- [3] P. Lawaetz, Phys. Rev. B **4**, 3460 (1971).
- [4] W. Lu, J. Xiang, B. P. Timko, Y. Wu, and C. M. Lieber, Proc. Natl. Acad. Sci. USA **102**, 10046 (2005).
- [5] J. M. Luttinger and W. Kohn, Phys. Rev. **97**, 869 (1955).
- [6] J. M. Luttinger, Phys. Rev. **102**, 1030 (1956).
- [7] L. J. Lauhon, M. S. Gudiksen, D. Wang, and C. M. Lieber, Nature (London) **420**, 57 (2002).
- [8] J. Xiang, W. Lu, Y. Hu, Y. Wu, H. Yan, and C. M. Lieber, Nature (London) **441**, 489 (2006).
- [9] J. Xiang, A. Vidan, M. Tinkham, R. M. Westervelt, and C. M. Lieber, Nat. Nanotech. **1**, 208 (2006).
- [10] Y. Hu, H. O. H. Churchill, D. J. Reilly, J. Xiang, C. M. Lieber, and C. M. Marcus, Nat. Nanotech. **2**, 622 (2007).
- [11] S. Roddaro, A. Fuhrer, P. Brusheim, C. Fasth, H. Q. Xu, L. Samuelson, J. Xiang, and C. M. Lieber, Phys. Rev. Lett. **101**, 186802 (2008).
- [12] K. M. Varahramyan, D. Ferrer, E. Tutuc, and S. K. Banerjee, Appl. Phys. Lett. **95**, 033101 (2009).
- [13] X.-J. Hao, T. Tu, G. Cao, C. Zhou, H.-O. Li, G.-C. Guo, W. Y. Fung, Z. Ji, G.-P. Guo, and W. Lu, Nano Lett. **10**, 2956 (2010).
- [14] H. Yan, H. S. Choe, S. Nam, Y. Hu, S. Das, J. F. Klemic, J. C. Ellenbogen, and C. M. Lieber, Nature (London) **470**, 240 (2011).
- [15] J. Nah, D. C. Dillen, K. M. Varahramyan, S. K. Banerjee, and E. Tutuc, Nano Lett. **12**, 108 (2012).
- [16] Y. Hu, F. Kuemmeth, C. M. Lieber, and C. M. Marcus, Nat. Nanotech. **7**, 47 (2012).
- [17] A. Blais, R.-S. Huang, A. Wallraff, S. M. Girvin, and R. J. Schoelkopf, Phys. Rev. A **69**, 062320 (2004).
- [18] A. Wallraff, D. I. Schuster, A. Blais, L. Frunzio, R.-S. Huang, J. Majer, S. Kumar, S. M. Girvin, and R. J. Schoelkopf, Nature (London) **431**, 162 (2004).
- [19] L. Frunzio, A. Wallraff, D. I. Schuster, J. Majer, and R. J. Schoelkopf, IEEE Transactions on Applied Superconductivity **15**, 860 (2005).
- [20] K. D. Petersson, L. W. McFaul, M. D. Schroer, M. Jung, J. M. Taylor, A. A. Houck, and J. R. Petta, Nature (London) **490**, 380 (2012).
- [21] V. Mourik, K. Zuo, S. M. Frolov, S. R. Plissard, E. P. A. M. Bakkers, and L. P. Kouwenhoven, Science **336**, 1003 (2012).
- [22] H. O. H. Churchill, V. Fatemi, K. Grove-Rasmussen, M. T. Deng, P. Caroff, H. Q. Xu, and C. M. Marcus, Phys. Rev. B **87**, 241401(R) (2013).
- [23] M. Trif, V. N. Golovach, and D. Loss, Phys. Rev. B **77**, 045434 (2008).
- [24] A. Imamoglu, D. D. Awschalom, G. Burkard, D. P. DiVincenzo, D. Loss, M. Sherwin, and A. Small, Phys. Rev. Lett. **83**, 4204 (1999).
- [25] A. Blais, J. Gambetta, A. Wallraff, D. I. Schuster, S. M. Girvin, M. H. Devoret, and R. J. Schoelkopf, Phys. Rev. A **75**, 032329 (2007).
- [26] A. Barenco, C. H. Bennett, R. Cleve, D. P. DiVincenzo, N. Margolus, P. Shor, T. Sleator, J. A. Smolin, and H. Weinfurter, Phys. Rev. A **52**, 3457 (1995).
- [27] D. Loss and D. P. DiVincenzo, Phys. Rev. A **57**, 120 (1998).
- [28] C. P. Slichter, *Principles of Magnetic Resonance* (Springer, Berlin, 1980).
- [29] V. N. Golovach, A. V. Khaetskii, and D. Loss, Phys. Rev. Lett. **93**, 016601 (2004).
- [30] M. Borhani, V. N. Golovach, and D. Loss, Phys. Rev. B **73**, 155311 (2006).
- [31] A. A. Clerk, M. H. Devoret, S. M. Girvin, F. Marquardt, and R. J. Schoelkopf, Rev. Mod. Phys. **82**, 1155 (2010).
- [32] J. B. Johnson, Phys. Rev. **32**, 97 (1928).
- [33] H. Nyquist, Phys. Rev. **32**, 110 (1928).
- [34] C. Fasth, A. Fuhrer, L. Samuelson, V. N. Golovach, and D. Loss, Phys. Rev. Lett. **98**, 266801 (2007).
- [35] S. Nadj-Perge, S. M. Frolov, E. P. A. M. Bakkers, and L. P. Kouwenhoven, Nature (London) **468**, 1084 (2010).
- [36] M. D. Schroer, K. D. Petersson, M. Jung, and J. R. Petta, Phys. Rev. Lett. **107**, 176811 (2011).
- [37] T. Meunier, I. T. Vink, L. H. Willems van Beveren, K.-J. Tielrooij, R. Hanson, F. H. L. Koppens, H. P. Tranitz, W. Wegscheider, L. P. Kouwenhoven, and L. M. K. Vandersypen, Phys. Rev. Lett. **98**, 126601 (2007).
- [38] F. Maier, C. Kloeffer, and D. Loss, Phys. Rev. B **87**, 161305(R) (2013).
